# Supplementary material for: Personalize Your LLM: Fake it then Align it
Source: arXiv:2503.01048 source file (2025-03-05)
Supplement: Supplementary file 1 [file process.tex]

\subsection{Process of Generating Insights and Self-Generated Preference Data}

The process of generating insight and preference data is illustrated in Figure \ref{fig:generate_pref_data}. We provide prompting details in Appendix \ref{appendix:prompt}.

\begin{figure*}[t!]
    \centering
    \hspace{-1cm}
    \includegraphics[width=1\textwidth]{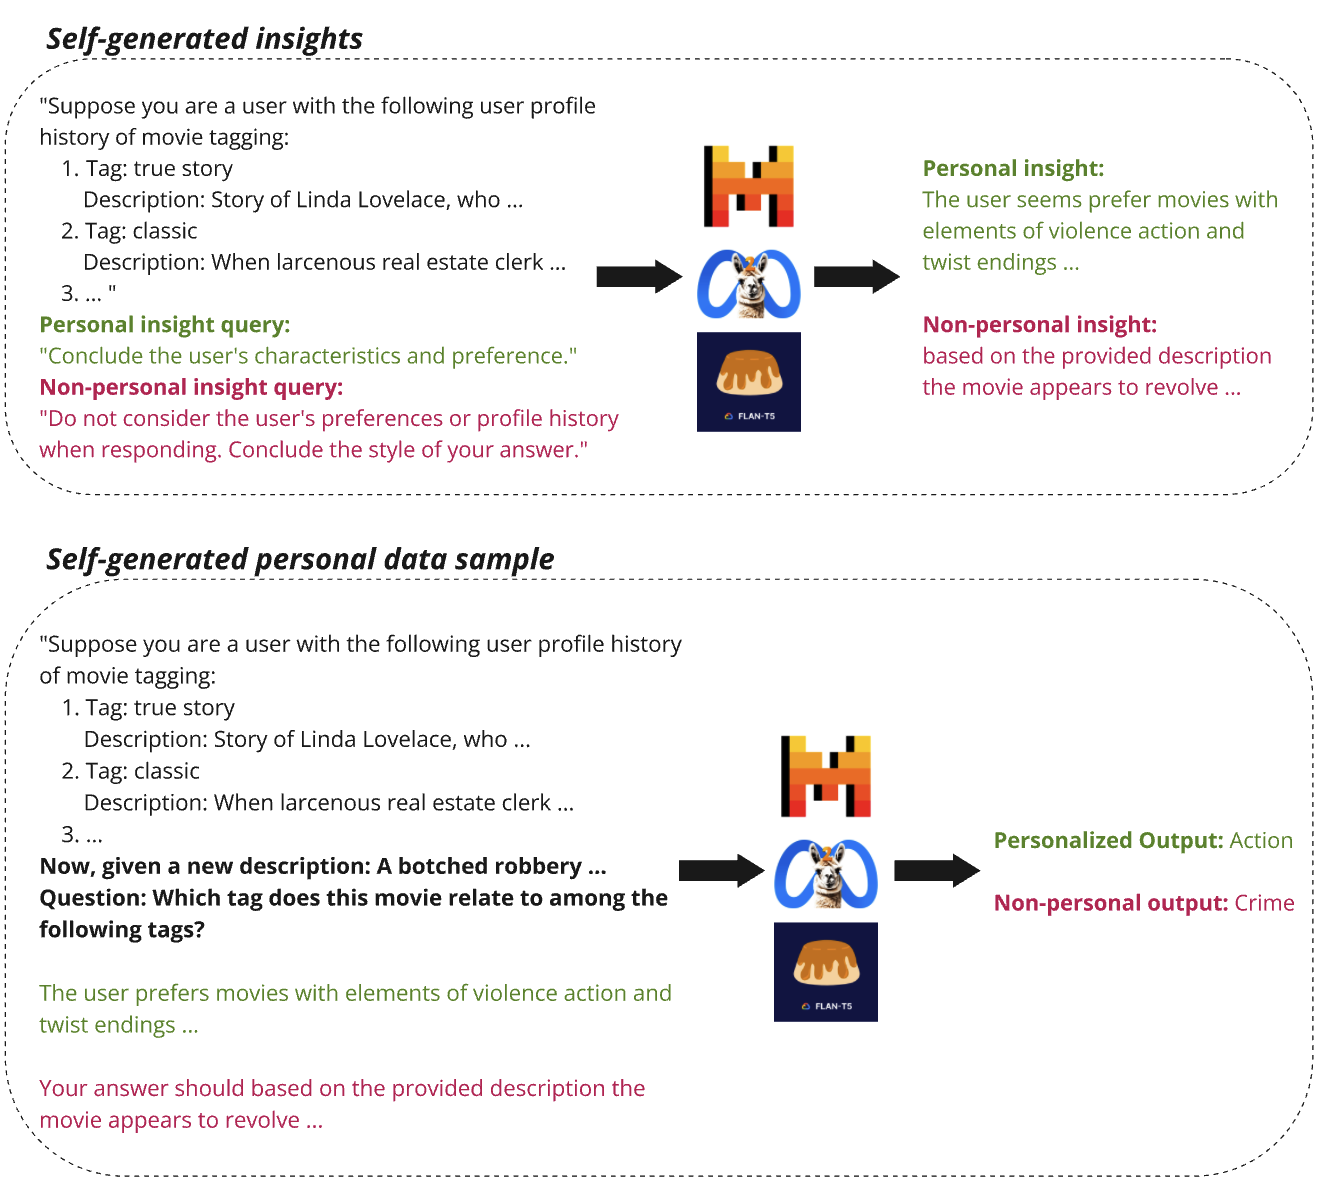}
    \caption{\SYSNAME}
    \label{fig:generate_pref_data}
\end{figure*}
